# Supplementary material for: Lie Detector: Unified Backdoor Detection via Cross-Examination Framework
Source: arXiv:2503.16872 source file (2025-04-01)
Supplement: Supplementary file 1 [file 7_appendix.tex]

\clearpage
\section{CKA Effectiveness Analysis}
To validate that CKA (Centered Kernel Alignment) effectively highlights differences between models and can distinguish clean models from backdoored ones, we select a specific poisoned dataset to test whether CKA values differ between two clean models versus those involving a backdoored model. This experiment aims to verify the discriminative capability of CKA in detecting backdoor attacks.

\begin{table}[h]
    \centering
    \caption{Comparison of CKA under different poisoned datasets}
     % 调整行间距
    \setlength{\tabcolsep}{10pt} % 调整列间距
    \small % 调整字体大小
    \begin{tabular}{l l c}
        \toprule
        \multicolumn{3}{c}{\textbf{poisoned data(poison rate=0.1)}} \\
        \midrule
        Model 1 & Model 2 & Similarity \\
        \midrule
        clean\_model\_1 & clean\_model\_2 & \cellcolor{yellow}{0.801} \\
        backdoor\_model\_1 & backdoor\_model\_2 & 0.311 \\
        backdoor\_model\_1 & backdoor\_model\_3 & 0.385 \\
        clean\_model\_1 & backdoor\_model\_1 & 0.254 \\
        clean\_model\_2 & backdoor\_model\_1 & 0.249 \\
        clean\_model\_1 & backdoor\_model\_2 & 0.267 \\
        clean\_model\_2 & backdoor\_model\_2 & 0.253 \\
        clean\_model\_1 & backdoor\_model\_3 & 0.368 \\
        clean\_model\_2 & backdoor\_model\_3 & 0.316 \\
        \midrule
        \multicolumn{3}{c}{\textbf{poisoned data(poison rate=0.05)}} \\
        \midrule
        clean\_model\_1 & clean\_model\_2 &\cellcolor{yellow}{0.801} \\
        backdoor\_model\_1 & backdoor\_model\_2 & 0.272 \\
        backdoor\_model\_1 & backdoor\_model\_3 & 0.324 \\
        clean\_model\_1 & backdoor\_model\_1 & 0.207 \\
        clean\_model\_2 & backdoor\_model\_1 & 0.209 \\
        clean\_model\_1 & backdoor\_model\_2 & 0.334 \\
        clean\_model\_2 & backdoor\_model\_2 & 0.29 \\
        clean\_model\_1 & backdoor\_model\_3 & 0.367 \\
        clean\_model\_2 & backdoor\_model\_3 & 0.328 \\
        \midrule
        \multicolumn{3}{c}{\textbf{poisoned data (poison rate=0.2)}} \\
        \midrule
        clean\_model\_1 & clean\_model\_2 &\cellcolor{yellow} {0.801} \\
        backdoor\_model\_1 & backdoor\_model\_2 & 0.286 \\
        backdoor\_model\_1 & backdoor\_model\_3 & 0.391 \\
        clean\_model\_1 & backdoor\_model\_1 & 0.263 \\
        clean\_model\_2 & backdoor\_model\_1 & 0.236 \\
        clean\_model\_1 & backdoor\_model\_2 & 0.229 \\
        clean\_model\_2 & backdoor\_model\_2 & 0.214 \\
        clean\_model\_1 & backdoor\_model\_3 & 0.351 \\
        clean\_model\_2 & backdoor\_model\_3 & 0.325 \\
        \bottomrule
    \end{tabular}

    \label{tab:poisoned_cka}
\end{table}

In \cref{tab:poisoned_cka}, we can see that there is a backdoor model, the CKA between the two models will be much lower than the CKA between two clean models, and this phenomenon is robust to changes in the poisoned rate. Additionally, we tested the trigger inversion capability of CKA on the CLIP.

We used the attack success rate as the metric to evaluate the capability of reverse trigger detection. Experimental results demonstrate that, compared to the four existing similarity measurement methods, our approach achieves the best performance in trigger inversion.

\section{Algorithm}

\begin{algorithm}[h]
\caption{Backdoor Detection and Trigger Optimization}
\label{alg:backdoor_detection}
\begin{algorithmic}[1]  % 1 表示显示行号
\For{epoch $e = 1$ to $epochs$}
    \State Adjust learning rate based on epoch $e$ and $args$
    \For{each batch $(clean\_x\_batch)$ in $clean\_train\_loader$}
        \State Generate poisoned batch $bd\_x\_batch$ using current trigger mask and patch
        \State Apply transformations to $clean\_x\_batch$ and $bd\_x\_batch$
        \State Compute activations for $model$ and $model1$ using $bd\_x\_batch$
        \State Compute CKA (Centered Kernel Alignment) between activations of $model$ and $model1$
        \State Compute loss components:
        \State \quad $loss\_cos$: CKA-based similarity loss
        \State \quad $loss\_reg$: Regularization loss (L2 norm of trigger mask)
        \State \quad $loss\_bias$: Bias loss to encourage high confidence in predictions
        \State \quad $loss\_uniformity$: Uniformity loss to encourage diverse predictions
        \State Combine losses: 
        \State \quad $loss = loss\_cos + loss\_reg \cdot loss\_lambda + loss\_bias + loss\_uniformity$
        \State Update trigger mask and patch using gradient descent
        \State Check for early stopping based on $loss\_cos$ and $loss\_reg$
        \If{early stopping condition met}
            \State \textbf{Break loop and return best trigger mask and patch}
        \EndIf
    \EndFor
    \State Log average losses for epoch $e$
    \State Save best trigger mask and patch if current results are better
\EndFor
\end{algorithmic}
\end{algorithm}

In \cref{tab:poisoned_cka}, we can see that there is a backdoor model, the CKA between the two models will be much lower than the CKA between two clean models, and this phenomenon is robust to changes in the poisoned rate. Additionally, we tested the trigger inversion capability of CKA on the CLIP.

We used the attack success rate as the metric to evaluate the capability of reverse trigger detection. Experimental results demonstrate that, compared to the four existing similarity measurement methods, our approach achieves the best performance in trigger inversion.

\section{Additional Details}
\subsection{Attack Setting}
\label{app:attack}
\textbf{Attack parameters}. Unless otherwise specified, all attack methods are configured with a 10\% poisoning rate, meaning 10\% of the training data is poisoned to simulate real-world adversarial conditions.
The number of backdoor training images used for poisoning was carefully chosen for each backdoor pattern and for each dataset to ensure a high attack success rate for the
created backdoor attacks. Details are shown in Tab.~\ref{tab:training_config}.
\begin{table}[t]
\centering
\caption{Training Configuration for Different Datasets and Models}
\label{tab:training_config}
\resizebox{0.48\textwidth}{!}{%
\begin{tabular}{|c|c|c|c|c|}
\hline
\textbf{Parameter} & \textbf{CIFAR-10} & \textbf{Tiniyimagenet} & \textbf{Caltech101} & \textbf{COCO} \\ \hline
Model & ResNet-18 & VGG-16 & CLIP & VLM \\ \hline
Optimizer & Adam & Adam & Adam & Adam \\ \hline
Batch Size & 128 & 128 & 224 & 224 \\ \hline
Epochs & 60 & 100 & 100 & 100 \\ \hline
Learning Rate & $1 \times 10^{-3}$ & $1 \times 10^{-4}$ & $1 \times 10^{-3}$ & $1 \times 10^{-3}$ \\ \hline
\end{tabular}}
\end{table}
\subsection{Defense Setting}
\label{app:defense}
\textbf{Detection protocol.} We evaluate each detection method under a semi-honest environment where only limited clean data is available for verification. Specifically, each dataset is split into a 90\%-10\% training-validation ratio, with only 10\% clean data accessible for detection. We report two key metrics: Detection Success Rate (DSR), which measures the percentage of correctly identified backdoored models, and False Positive Rate (FPR), which quantifies the rate of clean models misclassified as backdoored.

\textbf{Evaluation across learning paradigms.} To demonstrate the generalizability of our method, we test it across different learning paradigms. For supervised learning, we use ResNet18 and VGG16 trained on CIFAR-10 and TinyImageNet. For self-supervised learning, we evaluate CLIP and CoCoOp on ImageNet and Caltech101. For autoregressive learning, we test LLaVA and Mini-GPT4 on COCO and Flickr-30k.

\textbf{Implementation details.} All experiments are conducted using PyTorch, with models trained on NVIDIA A100 GPUs. For fair comparison, we fine-tune each detection method with hyperparameters optimized based on their respective papers.

\section{Method stability.}

\begin{figure}[htbp]
    \centering
    \begin{subfigure}{0.15\textwidth}
        \centering
        \includegraphics[width=\linewidth]{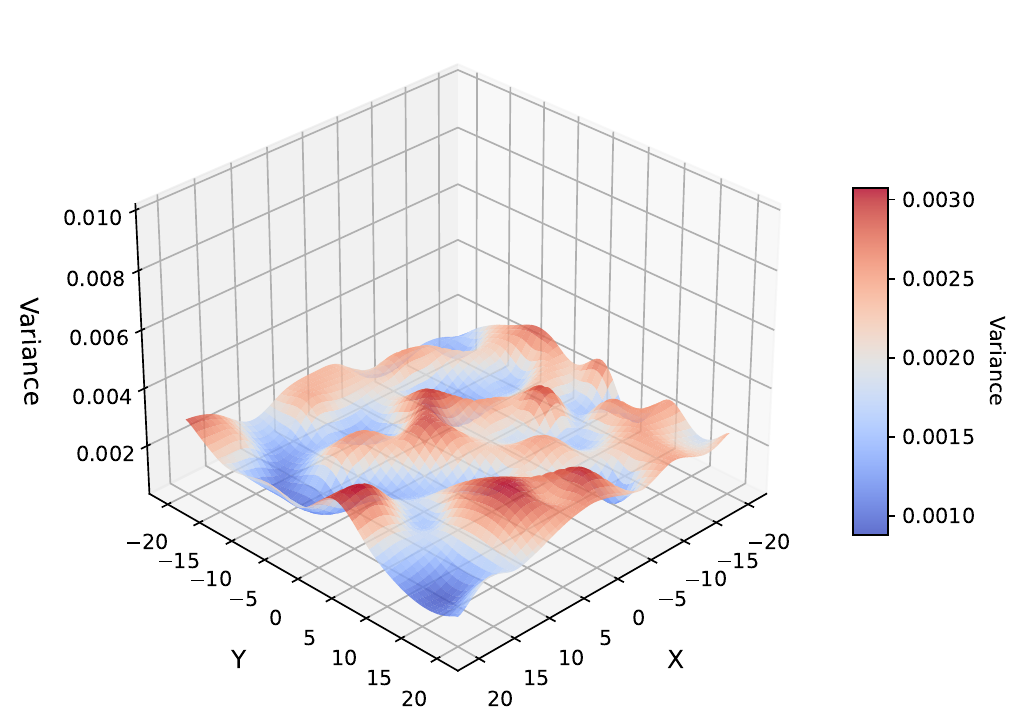}
        \caption{Lie Detector}
        \label{fig:rs18}
    \end{subfigure}
    \hfill
    \begin{subfigure}{0.15\textwidth}
        \centering
        \includegraphics[width=\linewidth]{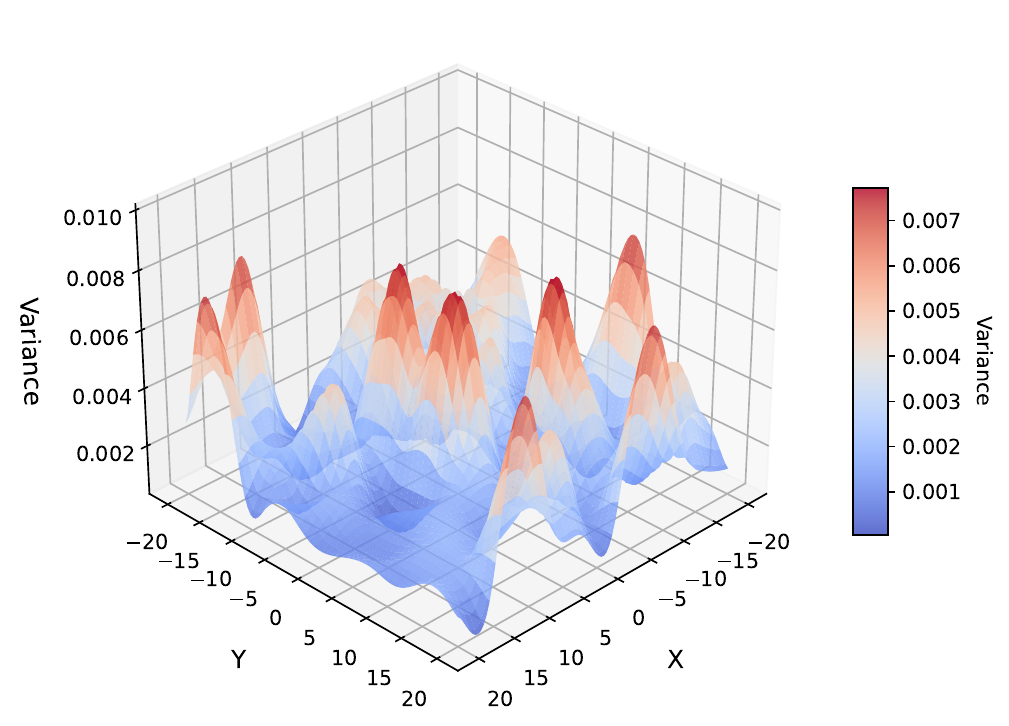}
        \caption{NAD}
        \label{fig:clip}
    \end{subfigure}
    \begin{subfigure}{0.15\textwidth}
        \centering
        \includegraphics[width=\linewidth]{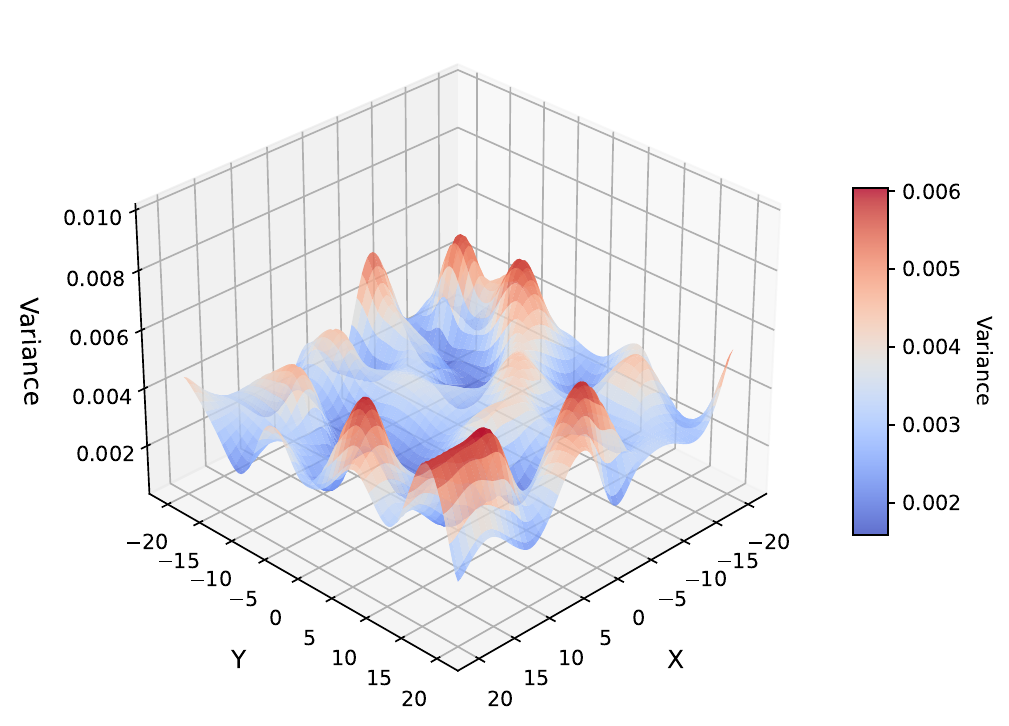}
        \caption{DECREE}
        \label{fig:clip}
    \end{subfigure}
    \caption{Stability of different defense methods on Belended.}
    \label{fig:method_stab}
\end{figure}

We conducted 10 experiments to obtain F1 scores, from which a variance was calculated. A total of 100 tests were performed, resulting in 10 sets of variances, which were used to evaluate the stability of the method, as shown in \cref{fig:method_stab}.

\section{Different Poisoning Rates.}

Next, we will discuss in depth the impact of some key factors on trigger reverse.
\begin{figure}[t]
    \vspace{0.3cm}
    \centering
    \begin{subfigure}{0.48\textwidth}
        \centering
        \includegraphics[width=0.9\linewidth]{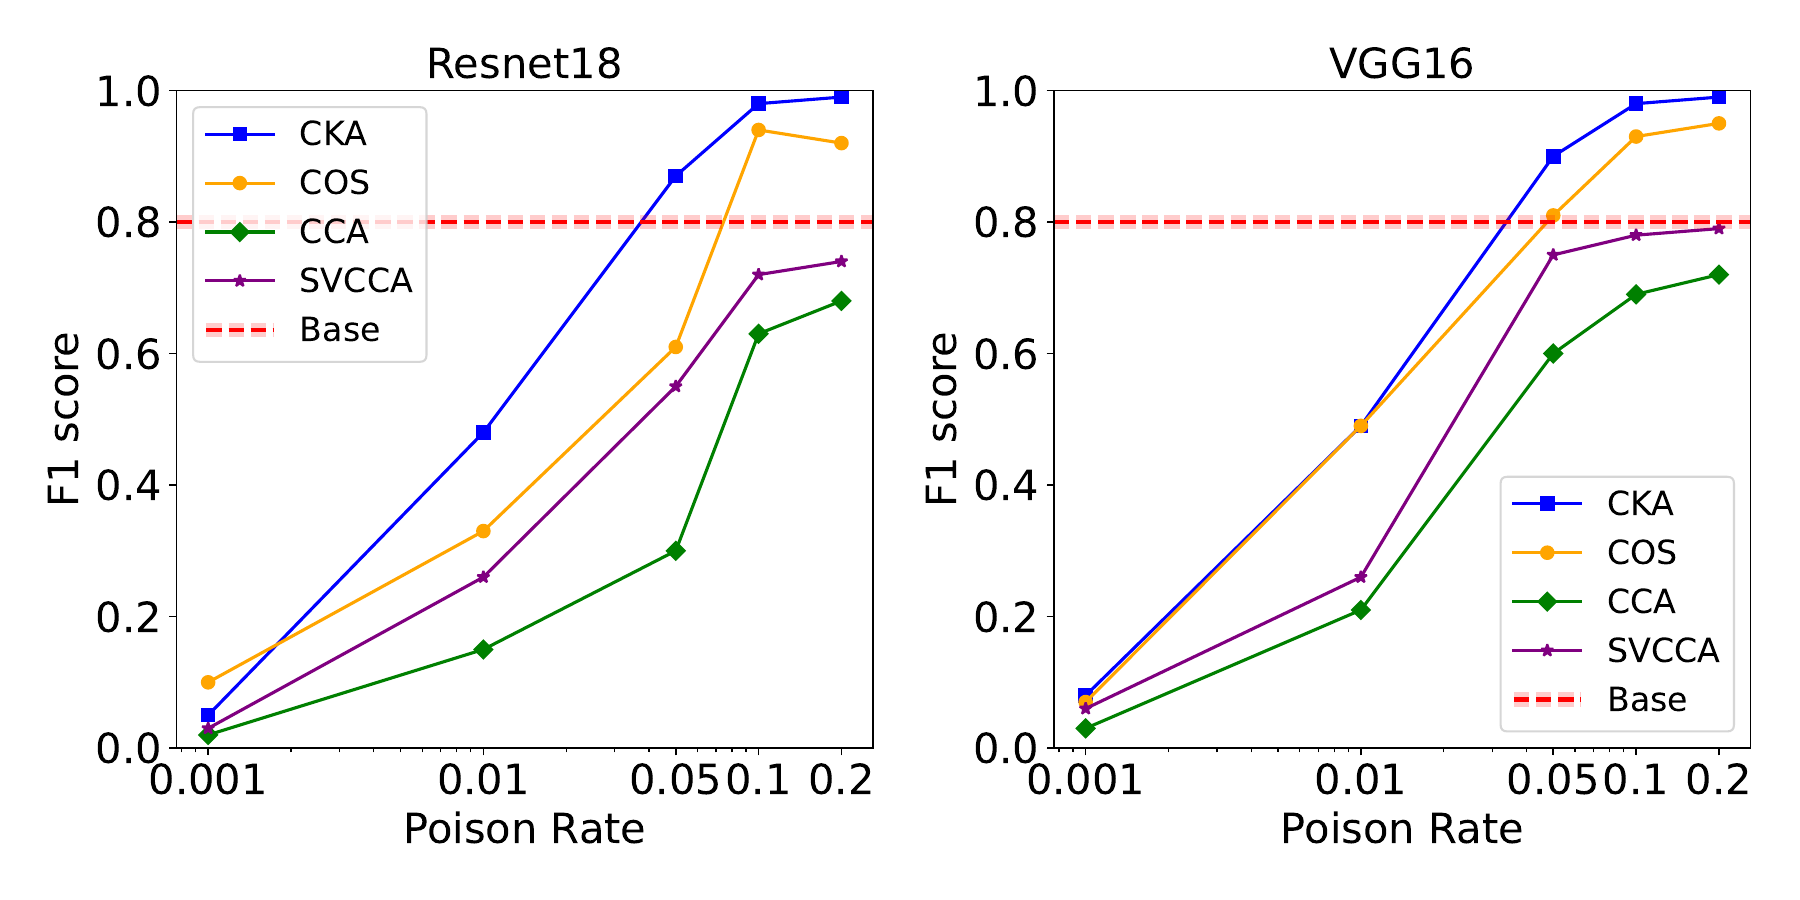}
        \vspace{-0.3cm}
        \caption{SL}
        \label{fig:rs18}
    \end{subfigure}
    \hfill
    \begin{subfigure}{0.48\textwidth}
        \centering
        \includegraphics[width=0.9\linewidth]{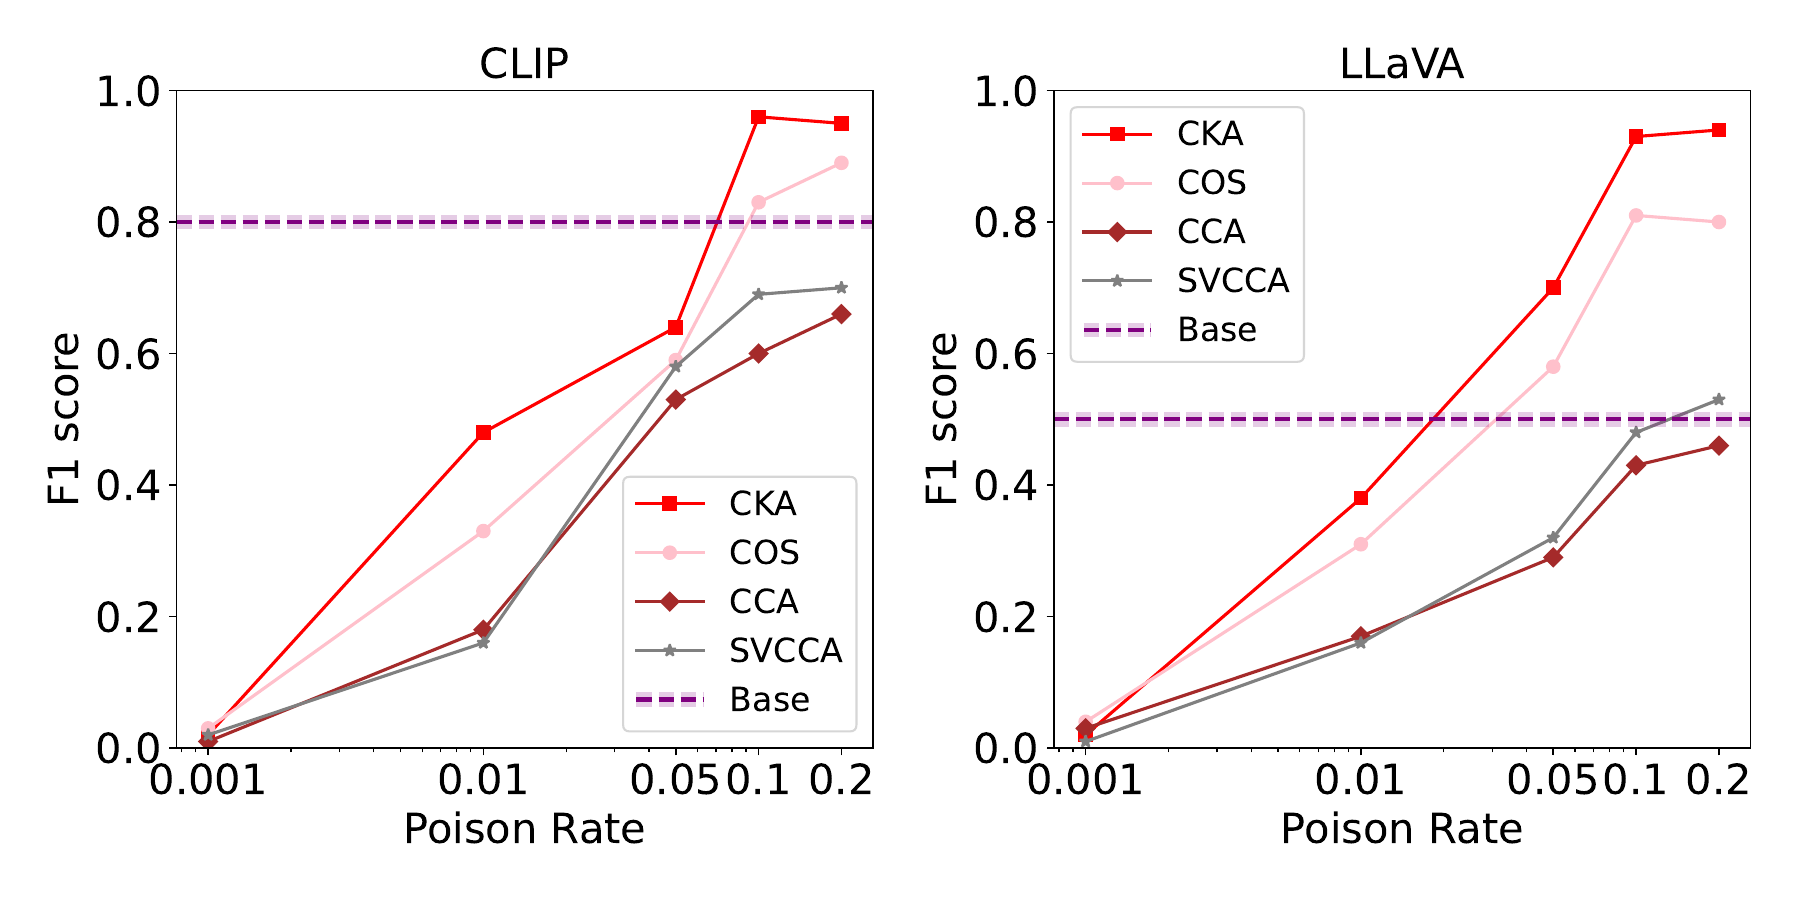}
        \vspace{-0.3cm}
        \caption{SSL and AL}
        \label{fig:clip}
    \end{subfigure}
    \vspace{-0.6cm}
    \caption{F1 scores under four different similarity metrics.}
    \label{fig:f1_four}
\vspace{-0.6cm}
\end{figure}
In \cref{fig:f1_four}, we present the F1 scores of four different similarity metrics across four model architectures under five poisoning rates (0.001\%, 0.01\%, 0.05\%, 0.1\%, and 0.2\%) against Blended attack. Higher F1 scores indicate a higher detection success rate. We draw the following conclusions: 1) CKA achieves the highest F1 scores across all architectures and poisoning rates, demonstrating its superior effectiveness in detecting backdoored models compared to other similarity metrics (COS, CCA, SVCCA). This highlights the robustness of CKA in capturing representation shifts caused by backdoor poisoning. 2) Detection performance improves as the poisoning rate increases, with all methods achieving higher F1 scores at higher poisoning levels. However, traditional metrics (COS, CCA, SVCCA) struggle at low poisoning rates, whereas CKA consistently performs well even in low-poisoning scenarios, further validating its reliability in identifying subtle backdoor patterns. 3) At extremely low poisoning rates (0.001\% and 0.01\%), detection performance is poor due to the weak backdoor effect and insufficient poisoned samples, leading to low F1 scores. Since the attack success rate (ASR) remains below 10-20\%, the model behaves similarly to a clean model, making it difficult for detection methods to effectively distinguish backdoored models. However, the low poisoning rate also implies that the attack itself is ineffective, limiting its practical threat.
